# Supplementary material for: Joint Optimization of Bit and Power Loading for Multicarrier Systems
Source: arXiv:1801.07571 source file (2019-02-08)
Supplement: Supplementary file 1 [file appendix_A.tex]

% !TEX root = Bedeer_WCL2013_0085.tex
\section*{Appendix A\\Proof of the KKT Conditions}

The KKT conditions are written as \cite{rao2009engineering}
\begin{IEEEeqnarray}{RCL}
\frac{\partial \mathcal{F}}{\partial \mathcal{P}_i} + \sum_{\varrho = 1}^{N}\lambda_{\varrho} \: \frac{\partial g_\varrho}{\partial \mathcal{P}_i} &{} = {}& 0, \label{eq:KH1}\\
\frac{\partial \mathcal{F}}{\partial b_i} +  \sum_{\varrho = 1}^{N}\lambda_\varrho \: \frac{\partial g_\varrho}{\partial b_i} &{} = {}& 0, \label{eq:KH2}\\
0.2 \exp\left(-1.6 \frac{\mathcal{C}_i \mathcal{P}_i}{2^{b_i} - 1}\right) - \textup{BER}_{th,i} & = & 0, \label{eq:KHnew}\\
\lambda_\varrho \left[0.2 \exp\left(-1.6 \frac{\mathcal{C}_i \mathcal{P}_i}{2^{b_i} - 1}\right) - \textup{BER}_{th,i}\right] & = & 0, \label{eq:KHnew1}\\
\lambda_\varrho &{} \geq {}& 0, \label{eq:KH3}
\end{IEEEeqnarray}
$\varrho = i = 1, ..., N$. One can show that these conditions are satisfied, as sketched in the proof below.

\textit{Proof of} (\ref{eq:KH1})-(\ref{eq:KH3}): (\ref{eq:KH1}) and (\ref{eq:KH2}) are satisfied from (\ref{eq:eq1}) and (\ref{eq:eq2}), respectively. Further, (\ref{eq:KHnew}) and (\ref{eq:KHnew1}) are satisfied from (\ref{eq:eq3}) and the discussion of \emph{case} 2 where the constraint on BER per subcarrier is always active, i.e., $\mathcal{Y}_i = 0$. From (\ref{eq:eq1}), one finds
\begin{IEEEeqnarray}{c}
\lambda_\varrho = \alpha \Bigg[ 0.2 \: \frac{1.6 \: \mathcal{C}_\varrho}{2^{b_\varrho}-1} \: \textup{exp}\Big(-1.6 \frac{\mathcal{C}_\varrho \mathcal{P}_\varrho}{2^{b_\varrho}-1}  \Big)  \Bigg]^{-1}, \label{eq:lambda}
\end{IEEEeqnarray}
which is non-negative for all values of $\varrho$, and hence it satisfies (\ref{eq:KH3}). \hfill$\blacksquare$ %\hfill$\square$ 
